# Supplementary material for: Consistency Diffusion Bridge Models
Source: arXiv:2410.22637 source file (2024-10-31)
Supplement: Supplementary file 1 [file AdditionalMetrics_ImageTranslation.tex]

\begin{table}[ht]   
    \centering
    \caption{Additional Metrics for Image-to-Image Translation Task}
    % \vskip 0.1in
    \resizebox{0.95\textwidth}{!}{% <------ Don't forget this %
    \begin{tabular}{lcccccccc}
    \toprule
    & \multicolumn{2}{c}{Edges$\to$Handbags ($64 \times 64$)}& \multicolumn{2}{c}{DIODE-Outdoor ($256 \times 256$)} \\ 
    \cmidrule(r){2-3} \cmidrule(l){4-5}
    & PSNR $\uparrow$ & SSIM $\uparrow$ & PSNR $\uparrow$ & SSIM $\uparrow$ \\
    \midrule
    DDBM~\cite{zhou2023denoising} (NFE=118)       & 8.36  & 0.29 & 22.64 & 0.63 \\
    \midrule
    DDBM (ODE-1, NFE=2)   & 30.67 & 0.91 & 25.32 & 0.75 \\
    DDBM (ODE-1, NFE=50)  & 29.10  & 0.89 & 23.52 & 0.70  \\
    DDBM (ODE-1, NFE=100) & 28.91 & 0.89 & 23.41 & 0.69 \\
    \midrule
    CBD (Ours, NFE=2)     & 25.25 & 0.84 & 22.68 & 0.65 \\
    CBT (Ours, NFE=2)     & 27.97 & 0.88 & 23.44 & 0.68  \\
    \bottomrule
    \end{tabular}% <------ Don't forget this %
    }
    % \vspace{-0.1in}
    \label{tab:AdditionalMetrics_ImageTranlation}
\end{table}
